# Supplementary material for: Diversity Augmentation of Dynamic User Preference Data for Boosting Personalized Text Summarizers
Source: arXiv:2510.10082 source file (2025-10-11)
Supplement: Supplementary file 1 [file Ethics.tex]

\section*{Ethics Statement}
We would like to declare that we used the PENS dataset and OpenAI (Reddit) dataset prepared and released by Microsoft Research/CAS and OpenAI respectively with complete compliance with the terms and conditions therein.
